# Supplementary material for: Uncertainty Quantification of DFT-predicted Finite Temperature Thermodynamic Properties within the Debye Model
Source: arXiv:1910.07891 source file (2019-10-04)
Supplement: Supplementary file 1 [file SI.pdf]

# Supporting Information For Uncertainty Quantification of Thermodynamic Modeling with the Debye model and DFT Calculations

Pinwen Guan,[†] Gregory Houchins,[‡,¶] and Venkatasubramanian Viswanathan[*,†,¶]

†*Department of Mechanical Engineering, Carnegie Mellon University, Pittsburgh, Pennsylvania 15213, USA*

‡*Wilton E. Scott Institute for Energy Innovation, Carnegie Mellon University, Pittsburgh, Pennsylvania 15213, USA*

¶*Department of Physics, Carnegie Mellon University, Pittsburgh, Pennsylvania 15213, US*

E-mail: venkvis@cmu.edu

## Determination of the scaling factor

The scaling factor used in the present work is determined from the Poisson ratio based on Eq. (...) in the main text, except for Mg, for which the default value $s = 0.617$ works quite well. The Poisson ratio is taken from the Materials Project as 0.37 for Al, 0.31 for Ca, 0.36 for Li, 0.24 for Al2O3, 0.23 for GaAs, 0.16 for Li2O and 0.35 for NiO.

# Gibbs Free Energy at Finite Pressure

The Gibbs energy around zero pressure can be expanded as

$$G(P,T) = F(V(P,T),T) + PV = F(V(0,T),T) + \left.\frac{\partial F}{\partial P}\right|_{P=0,T} P + \left.\frac{\partial^2 F}{\partial P^2}\right|_{P=0,T} P^2 + ... + PV$$

where

$$\left.\frac{\partial F}{\partial P}\right|_{P=0,T} = \left.\frac{\partial F}{\partial V}\right|_{V(P=0,T),T} \left.\frac{\partial V}{\partial P}\right|_{P=0,T} = -P\Big|_{V(P=0,T),T} \left.\frac{\partial V}{\partial P}\right|_{P=0,T} = 0$$

$$\begin{aligned}\left.\frac{\partial^2 F}{\partial P^2}\right|_{P=0,T} &= \frac{\partial}{\partial V}[\frac{\partial F}{\partial V}(\frac{\partial P}{\partial V})^{-1}]\Big|_{V(P=0,T),T} (\frac{\partial P}{\partial V})^{-1}\Big|_{V(P=0,T),T} \\ &= \frac{\partial}{\partial V}[P(\frac{\partial P}{\partial V})^{-1}]\Big|_{V(P=0,T),T} (\frac{\partial^2 F}{\partial V^2})^{-1}\Big|_{V(P=0,T),T} \\ &= \frac{\partial P}{\partial V}(\frac{\partial P}{\partial V})^{-1}\Big|_{V(P=0,T),T} \frac{V(P=0,T)}{B(P=0,T)} = \frac{V(P=0,T)}{B(P=0,T)}\end{aligned}$$

At ambient conditions where P is small, the deviation of $G(P,T)$ from $G(P=0,T)$ is

$$G(P,T) - G(P=0,T) \approx \frac{V(P=0,T)}{B(P=0,T)} P^2 + PV \approx PV(1 + \frac{P}{B(P=0,T)}) \approx PV$$

which is negligible, therefore the pressure effect can be ignored and it is valid to use Gibbs energy at zero pressure

# Other Materials Tested

Here we present the rest of the predictions of thermodynamic properties and their uncertainties for the other materials test. The include Ca, Al, GaAs, and NiO shown in Figurew S1,S2, S3, and S4 respectively. As breifely mentioned within the main text, these materials

largely show good agreement with experiment as well as low prediction uncertainty.

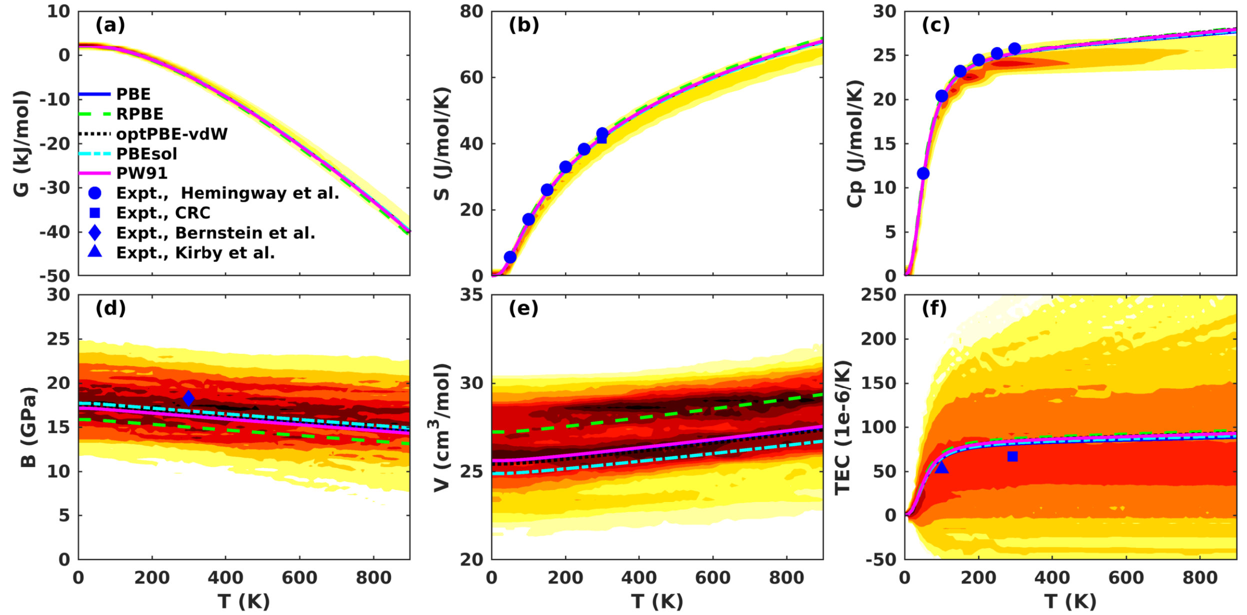


Figure S1: Thermodynamic properties of fcc Ca: (a) Gibbs energy (b) entropy (c) isobaric heat capacity (d) bulk modulus (e) volume and (f) volumetric thermal expansion coefficient from DFT Debye calculations compared with experimental data in the literature.[1–4] The colormap represents the PDF of each property calculated by BEEF. The colormap represents the PDF of each property calculated by BEEF. The natural logarithm of PDF is presented in (f) for better view.

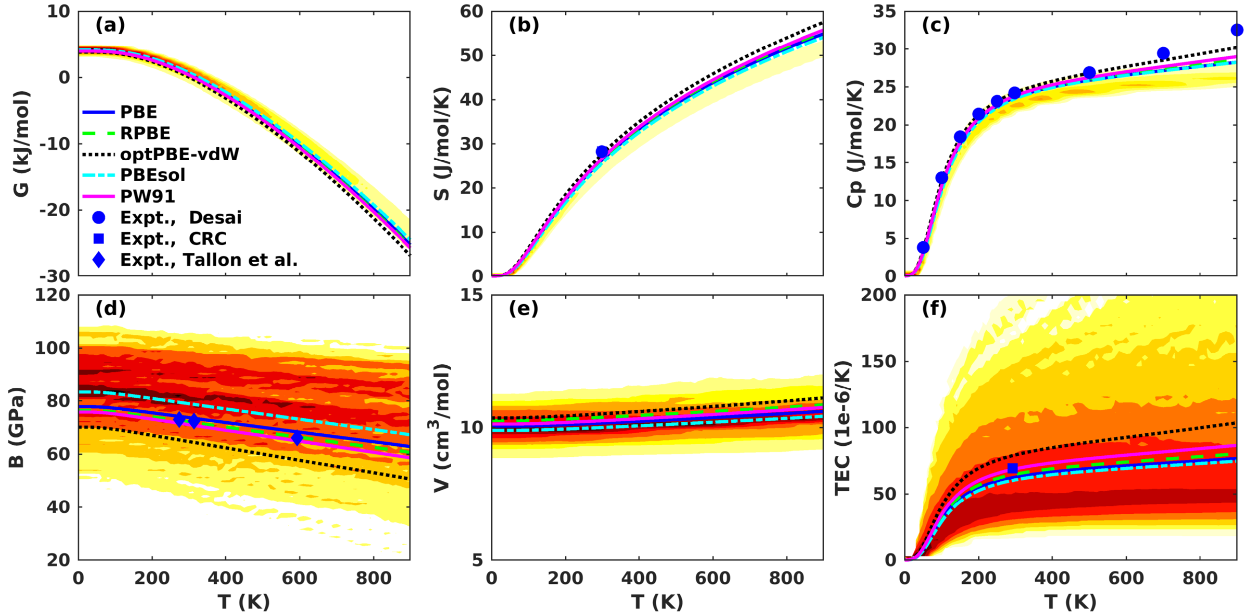


Figure S2: Thermodynamic properties of fcc Al: (a) Gibbs energy (b) entropy (c) isobaric heat capacity (d) bulk modulus (e) volume and (f) volumetric thermal expansion coefficient from DFT Debye calculations compared with experimental data in the literature.[2,5,6] The colormap represents the PDF of each property calculated by BEEF. The colormap represents the PDF of each property calculated by BEEF. The natural logarithm of PDF is presented in (f) for better view.

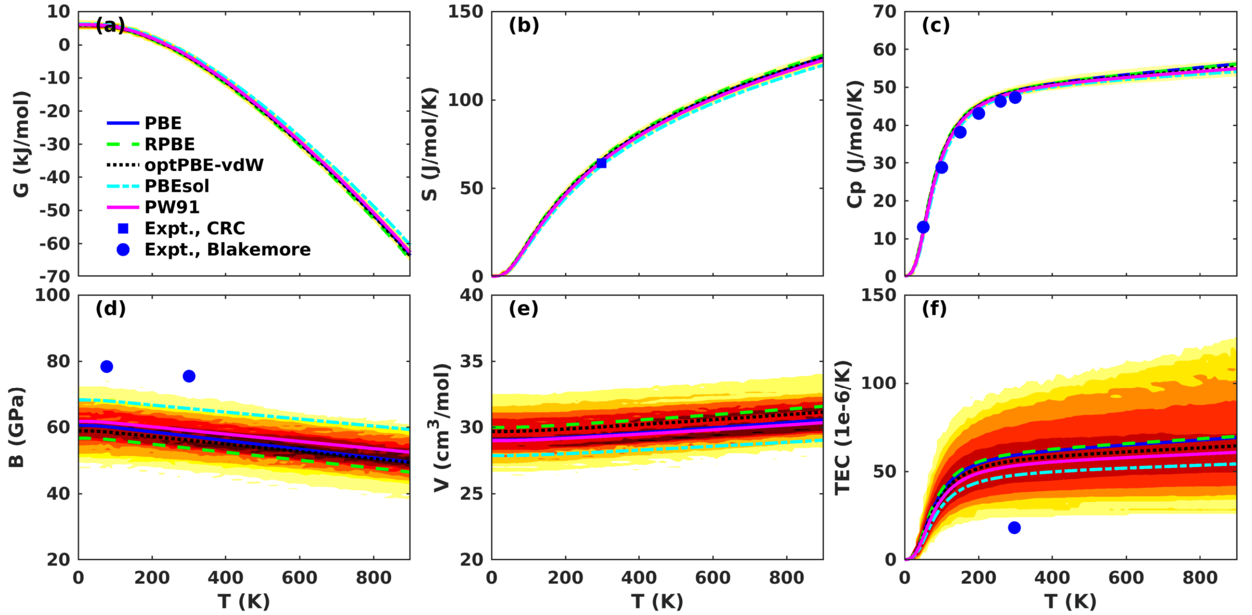


Figure S3: Thermodynamic properties of zincblende GaAs: (a) Gibbs energy (b) entropy (c) isobaric heat capacity (d) bulk modulus (e) volume and (f) volumetric thermal expansion coefficient from DFT Debye calculations compared with experimental data in the literature.[2,7] The colormap represents the PDF of each property calculated by BEEF. The colormap represents the PDF of each property calculated by BEEF. The natural logarithm of PDF is presented in (f) for better view.

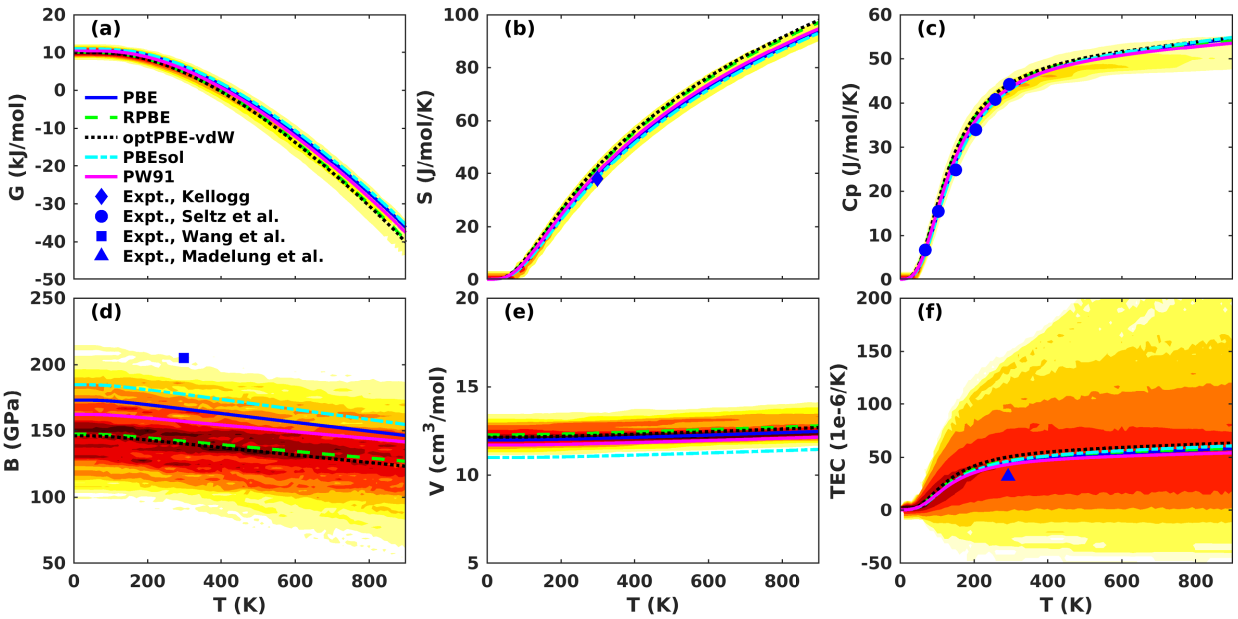


Figure S4: Thermodynamic properties of rocksalt NiO: (a) Gibbs energy (b) entropy (c) isobaric heat capacity (d) bulk modulus (e) volume and (f) volumetric thermal expansion coefficient from DFT Debye calculations compared with experimental data in the literature.[8–11] The colormap represents the PDF of each property calculated by BEEF. The colormap represents the PDF of each property calculated by BEEF. The natural logarithm of PDF is presented in (f) for better view.

We also include for comparison with the table of statistics included in the main text, the mean ($\mu$), standard deviation ($\sigma$), coefficient of variation (COV), skew, and excess kurtosis in Table S1 of the predictions of all properties at 900 K, except in the case of Li, which is for 450K as 900K is well above the melting point of Li. The corresponding predictions of the other GGA level functions are also shown.

# Distributions of Thermodynamic Properties

As was shown in the main text for NiO at 300K, we include here the empirical distributions of NiO at 900K in Figure S5 as well as Al at 300K and 900K in Figures S6 and S7, and Al2O3 at 300K and 900K in Figures S8 and S9.

Table S1: Properties and their statistics at high temperature (450 K for Li and 900 K for the others).

| | Prop. | PBE | RPBE | optPBE-vdW | PBEsol | PW91 | BEEF-vdW | $\mu$ | $\sigma$ | COV | Skew | Kurt |
|---|---|---|---|---|---|---|---|---|---|---|---|---|
| Al | G | -25.21 | -25.43 | -26.85 | -24.49 | -25.71 | -24.35 | -24.97 | 3.07 | | -1.22 | 1.59 |
| | S | 54.91 | 55.27 | 57.5 | 54.12 | 55.76 | 53.43 | 54.83 | 4.81 | 0.09 | 1.7 | 3.67 |
| | Cp | 28.25 | 28.54 | 30.2 | 28.23 | 28.99 | 27.05 | 29.0 | 5.35 | 0.18 | 6.38 | 77.21 |
| | BT | 62.83 | 60.65 | 50.65 | 67.27 | 58.59 | 70.4 | 67.16 | 20.71 | 0.31 | -0.52 | -0.25 |
| | VT | 10.61 | 10.85 | 11.11 | 10.42 | 10.75 | 10.51 | 10.7 | 0.92 | 0.09 | 1.01 | 1.56 |
| | TEC | 76.67 | 80.18 | 103.53 | 74.7 | 86.57 | 59.43 | 84.42 | 67.55 | 0.8 | 4.09 | 23.73 |
| Ca | G | -40.07 | -40.85 | -39.99 | -39.85 | -40.15 | -39.82 | -39.6 | 2.67 | | -0.64 | 0.59 |
| | S | 70.9 | 71.95 | 70.96 | 70.7 | 71.11 | 70.36 | 70.77 | 4.49 | 0.06 | 1.44 | 2.92 |
| | Cp | 27.7 | 28.1 | 28.02 | 27.8 | 27.95 | 27.12 | 29.06 | 6.31 | 0.22 | 3.3 | 13.83 |
| | BT | 14.53 | 13.12 | 14.51 | 14.9 | 14.3 | 14.97 | 15.14 | 4.38 | 0.29 | -0.24 | 0.32 |
| | VT | 27.45 | 29.35 | 27.35 | 26.71 | 27.55 | 27.91 | 27.95 | 2.33 | 0.08 | -0.15 | 0.56 |
| | TEC | 88.53 | 96.21 | 93.74 | 90.25 | 93.01 | 77.23 | 94.41 | 104.11 | 1.1 | 2.65 | 10.6 |
| Li | G | -6.41 | -6.27 | -6.36 | -6.38 | -6.33 | -5.7 | -5.2 | 1.44 | | -0.32 | 0.35 |
| | S | 42.07 | 41.52 | 41.84 | 41.83 | 41.66 | 40.59 | 39.07 | 3.54 | 0.09 | 0.56 | 0.36 |
| | Cp | 28.6 | 28.02 | 28.32 | 28.23 | 28.09 | 28.57 | 27.45 | 2.97 | 0.11 | 0.02 | 7.8 |
| | BT | 10.55 | 10.86 | 10.68 | 10.73 | 10.85 | 12.03 | 13.91 | 3.87 | 0.28 | 0.38 | 0.21 |
| | VT | 13.7 | 14.09 | 13.87 | 13.65 | 13.69 | 13.16 | 13.08 | 1.36 | 0.1 | 0.36 | -0.03 |
| | TEC | 256.4 | 232.38 | 245.41 | 243.87 | 237.79 | 246.27 | 188.86 | 117.07 | 0.62 | 0.22 | 0.29 |
| Mg | G | -34.38 | -34.55 | -34.7 | -33.49 | -34.24 | -33.89 | -33.87 | 1.86 | | -0.85 | 2.1 |
| | S | 65.48 | 65.46 | 65.8 | 64.05 | 65.1 | 64.65 | 64.79 | 2.88 | 0.04 | 1.54 | 5.15 |
| | Cp | 29.6 | 29.11 | 29.53 | 28.56 | 29.07 | 28.92 | 29.43 | 3.02 | 0.1 | 2.96 | 17.34 |
| | BT | 27.22 | 26.99 | 26.43 | 30.6 | 28.02 | 28.92 | 29.19 | 5.88 | 0.2 | -0.4 | 0.75 |
| | VT | 15.12 | 15.52 | 15.34 | 14.68 | 15.06 | 15.17 | 15.22 | 0.86 | 0.06 | 0.99 | 4.54 |
| | TEC | 113.31 | 106.31 | 113.22 | 95.94 | 105.43 | 101.56 | 107.12 | 46.76 | 0.44 | 2.97 | 20.48 |
| NiO | G | -36.23 | -39.55 | -40.06 | -35.47 | -37.57 | -39.94 | -39.55 | 4.45 | | -0.42 | 0.55 |
| | S | 93.81 | 97.11 | 97.97 | 93.16 | 94.78 | 97.97 | 97.91 | 6.77 | 0.07 | 0.99 | 1.51 |
| | Cp | 54.56 | 54.11 | 54.82 | 54.89 | 53.6 | 55.09 | 56.37 | 8.7 | 0.15 | 1.68 | 7.48 |
| | BT | 146.29 | 126.94 | 123.25 | 154.59 | 141.53 | 123.1 | 126.44 | 31.62 | 0.25 | -0.07 | 0.03 |
| | VT | 12.46 | 12.77 | 12.67 | 11.44 | 12.13 | 12.76 | 12.75 | 0.73 | 0.06 | 0.47 | 0.5 |
| | TEC | 57.99 | 58.3 | 63.34 | 60.7 | 54.09 | 64.67 | 64.9 | 51.04 | 0.79 | 1.46 | 3.65 |
| GaAs | G | -63.54 | -64.77 | -63.74 | -60.47 | -62.69 | -63.71 | -31.67 | 1.14 | | -0.27 | 1.11 |
| | S | 123.88 | 125.2 | 123.77 | 119.63 | 122.4 | 123.82 | 61.76 | 1.51 | 0.02 | 0.82 | 2.07 |
| | Cp | 56.14 | 56.09 | 55.38 | 54.15 | 54.92 | 55.57 | 27.93 | 1.35 | 0.05 | 1.54 | 5.7 |
| | BT | 49.49 | 46.5 | 49.34 | 59.28 | 52.45 | 49.36 | 50.3 | 6.06 | 0.12 | -0.09 | 1.71 |
| | VT | 30.56 | 31.57 | 31.14 | 29.02 | 30.34 | 30.97 | 15.47 | 0.78 | 0.05 | 0.28 | 0.32 |
| | TEC | 69.12 | 69.81 | 64.44 | 54.25 | 60.8 | 65.65 | 66.14 | 17.03 | 0.26 | 1.21 | 4.27 |
| $Li_2O$ | G | -24.04 | -33.45 | -30.34 | -28.21 | -29.82 | -26.25 | -23.19 | 9.88 | | -0.3 | 0.18 |
| | S | 112.7 | 125.96 | 122.5 | 119.24 | 121.24 | 115.76 | 112.88 | 15.94 | 0.14 | 0.85 | 0.47 |
| | Cp | 87.84 | 97.34 | 96.57 | 93.76 | 94.72 | 89.92 | 92.49 | 24.38 | 0.26 | 1.88 | 3.52 |
| | BT | 56.8 | 38.39 | 42.65 | 47.6 | 44.71 | 51.05 | 58.96 | 22.6 | 0.38 | 0.23 | -0.14 |
| | VT | 16.77 | 19.31 | 18.51 | 17.22 | 17.74 | 18.12 | 17.84 | 1.52 | 0.09 | 0.47 | 0.02 |
| | TEC | 135.28 | 191.14 | 182.99 | 169.42 | 175.61 | 145.17 | 145.28 | 130.79 | 0.9 | 1.6 | 3.02 |
| $Al_2O_3$ | G | -25.97 | -33.55 | -30.21 | -26.71 | -29.15 | -31.96 | -31.58 | 5.7 | | -0.07 | -0.09 |
| | S | 164.82 | 173.38 | 169.74 | 165.85 | 168.63 | 171.84 | 171.5 | 7.25 | 0.04 | 0.6 | 0.92 |
| | Cp | 125.83 | 128.71 | 127.74 | 126.54 | 127.51 | 128.65 | 128.76 | 5.54 | 0.04 | 1.74 | 5.65 |
| | BT | 207.54 | 177.4 | 189.39 | 204.0 | 193.74 | 182.85 | 185.27 | 22.73 | 0.12 | -0.03 | 0.09 |
| | VT | 27.32 | 28.85 | 28.34 | 27.43 | 27.98 | 28.48 | 28.4 | 1.1 | 0.04 | -0.07 | -0.46 |
| | TEC | 38.59 | 45.71 | 43.18 | 40.35 | 42.67 | 45.51 | 44.94 | 13.29 | 0.3 | 1.07 | 3.41 |

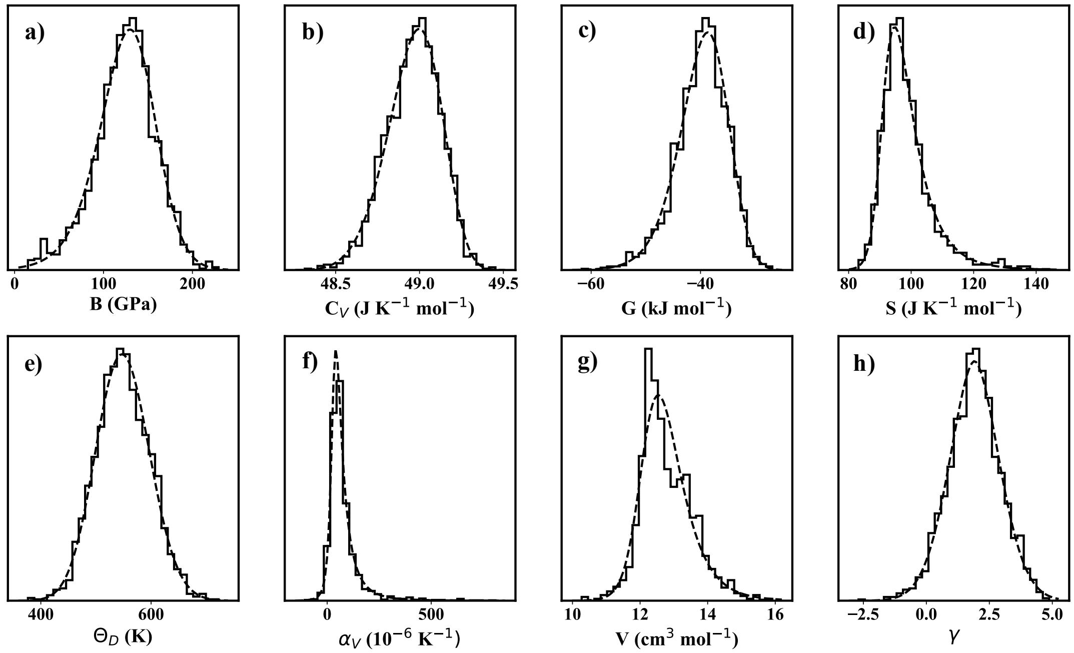


Figure S5: Distribution of thermodynamic properties of rocksalt NiO at 900 K

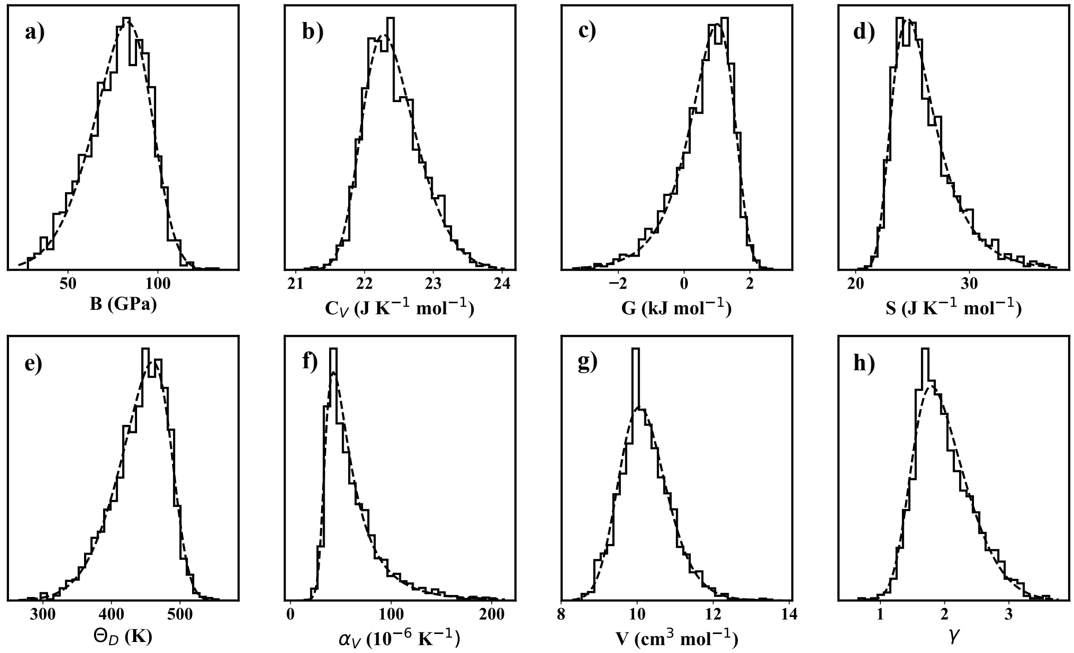


Figure S6: Distribution of thermodynamic properties of fcc Al at 300 K

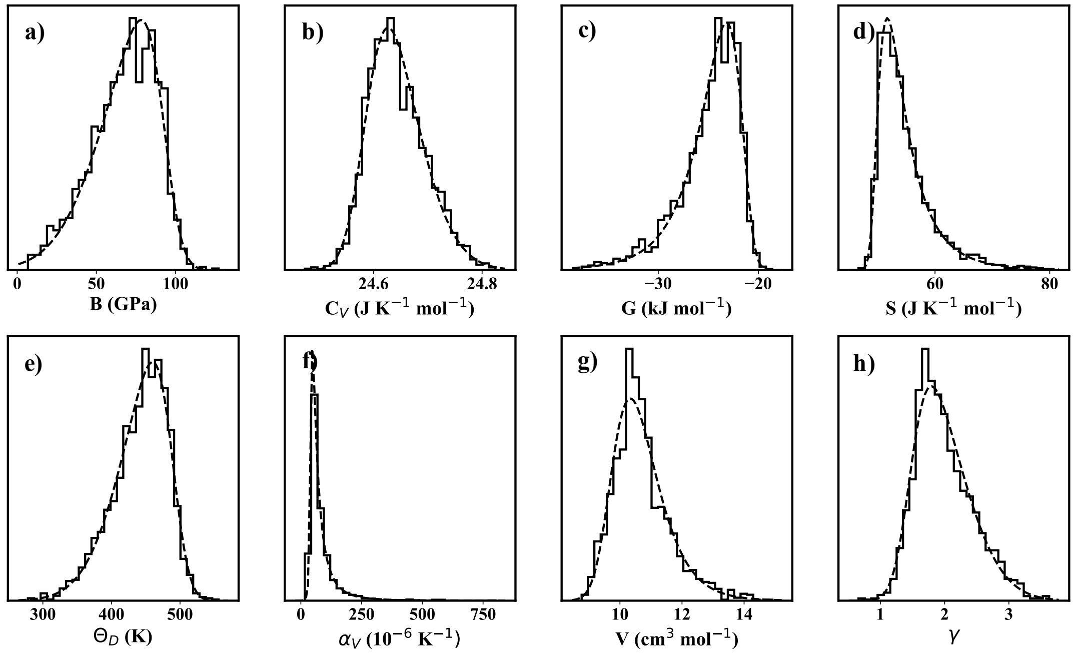


Figure S7: Distribution of thermodynamic properties of fcc Al at 900 K

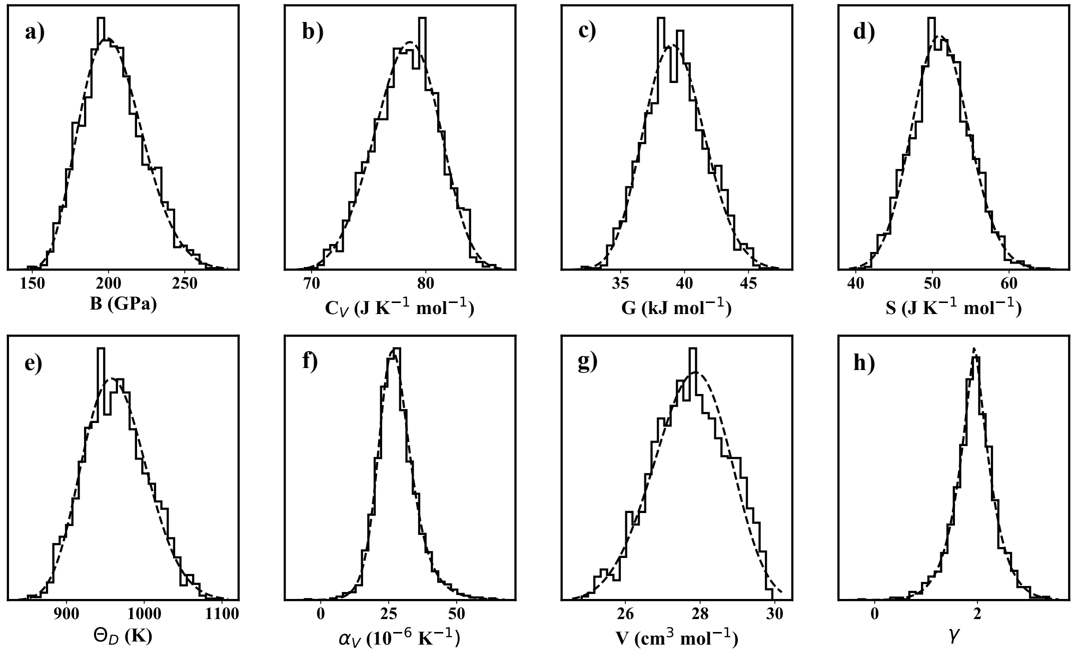


Figure S8: Distribution of thermodynamic properties of corundum Al2O3 at 300 K

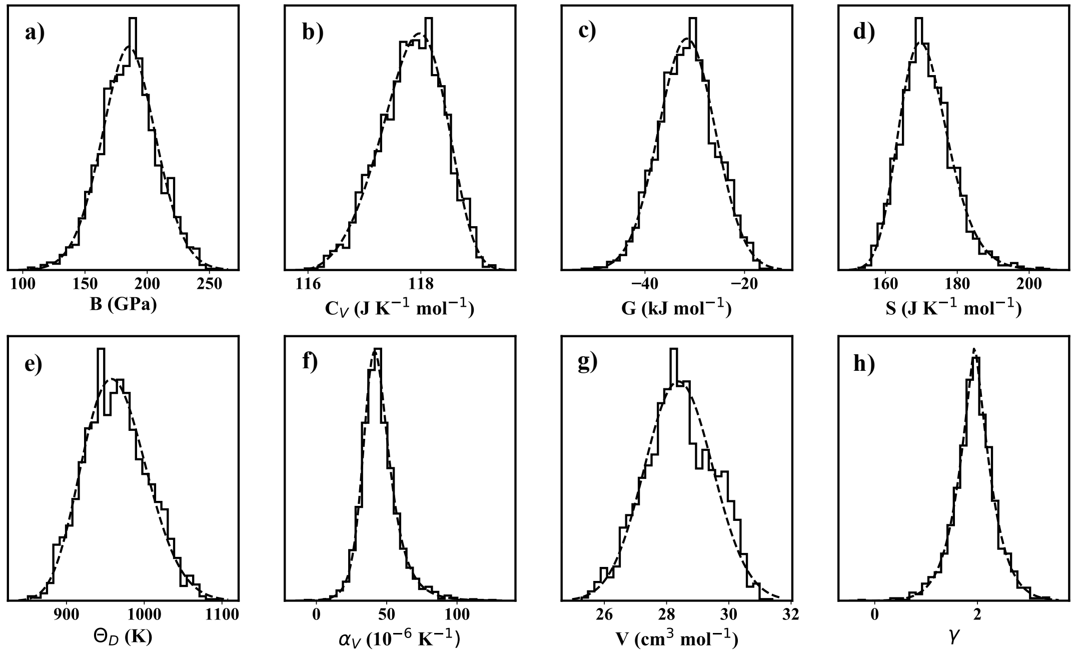


Figure S9: Distribution of thermodynamic properties of corundum Al2O3 at 900 K

# Statistical Model Fitting

The Cramer-von Mises criteron, $\omega^2$ for testing that a set of data $x_1, x_2, \cdot x_N$ has been drawn from a model distribution $F(y)$ is given by

$$\omega^2 = \int_{-\infty}^{\infty} [F_N(y) - F(y)]^2 \mathrm{d}F(y)$$

where $F_N(y)$ is the empirical distribution function defined as the number of samples in the set of data that are less than or equal to y divided by the total number of samples:

$$F_N(y) = \frac{1}{N} \sum_{i=1}^{N} \mathbf{1}_{X_i \leq y}$$

where $\mathbf{1}_{X_i \leq y}$ is the indicator function that is 1 if the inequality is true and 0 if false.

The limiting distribution of this statistic in the case of the samples being drawn from the

model distribution is given by[12]

$$N\omega^2 = \frac{1}{12N} + \sum_{i=1}^{N} \left( F(x_i) - \frac{2i-1}{2N} \right)^2$$

The computed statistic for the set of data being tested can then be compared to this limiting distribution and a statistical conclusion can be made.

[13]

# References


(1) Hemingway, B. S.; Robie, R. A.; Chase, M. W. Molar heat capacity and entropy of calcium metal. *The Journal of Chemical Thermodynamics* **1997**, *29*, 211 – 220.

(2) CRC handbook of chemistry and physics. c1977-.

(3) Bernsztejn, M.; Zajmowskij, W. Struktura i własnosci mechaniczne metali (Structure and Mechanical Properties of Metals). 1973.

(4) R. K. Kirby,, T. A. Hahn,, Rothrock, B. D., Eds. *American Institute of Physics Handbook*; McGraw-Hill: New York, 1972.

(5) Desai, P. D. Thermodynamic properties of aluminum. *International Journal of Thermophysics* **1987**, *8*, 621–638.

(6) Tallon, J.; Wolfenden, A. Temperature dependence of the elastic constants of aluminum. *Journal of Physics and Chemistry of Solids* **1979**, *40*, 831–837.

(7) Blakemore, J. S. Semiconducting and other major properties of gallium arsenide. *Journal of Applied Physics* **1982**, *53*, R123–R181.

(8) Kellogg, H. H. Thermodynamic properties of the oxides of copper and nickel. *Journal of Chemical & Engineering Data* **1969**, *14*, 41–44.

Table S2: The fit for the properties of $Al_2O_3$ at 300K with the result of the Cramer von Mises (CVM) goodness of fit test. This is the chance of error when rejecting the null hypothesis that the data we have was drawn from the model distribution. If this is above 0.05 we say there is no statistically significant evidence that the model distribution and real distribution of the data are different. The result of the Vuong test for comparing the two best distributions is also shown. This is is the chance of error that when assuming the chosen distribution is better than the second best distribution at describing the data. If this is below 0.05, we say there is enough statistical evidence to conclude the chosen model is closer to the true data generation process than the second best model. Here $\phi(x)$ is the normal pdf and $\Phi(x)$ is the normal cdf.

| Property | Form | | CVM | Vuong Test |
|---|---|---|---|---|
| $B_T$ | $f(y,c) = c\phi(y)\Phi(-y)^{c-1}$ | $c = 0.1157$, $y = \dfrac{x - 175.9}{9.314}$ | 0.84 | 0.020 |
| $C_V$ | $f(y,c) = cx^{c-1}\exp -x^c$ | $c = 4.274$, $y = \dfrac{x - 67.74}{11.57}$ | 0.87 | $6.1\times10^{-6}$ |
| $G$ | $f(y,c) = c\phi(y)\Phi(-y)^{c-1}$ | $c = 0.3548$, $y = \dfrac{x - 637.40}{1.684}$ | 0.78 | $8.3\times10^{-5}$ |
| $S$ | $f(y,c) = 2\phi(y)\Phi(cy)$ | $c = 0.8940$, $y = \dfrac{x - 48.77}{4.418}$ | 0.87 | 0.16 |
| $\Theta_D$ | $f(y,c) = c\phi(y)\Phi(-y)^{c-1}$ | $c = 0.2561$, $y = \dfrac{x - 923.3}{25.80}$ | 0.82 | $2.6\times10^{-3}$ |
| $\alpha_V$ | $f(y,a,c) = \dfrac{c}{\sqrt{y^2+1}}\phi(a + c\sinh^{-1}(y))$ | $a = -0.6976$, $c = 1.784$, $y = \dfrac{x - 23.25}{10.45}$ | 0.99 | $1.1\times10^{-5}$ |
| $V$ | $f(y,c) = cx^{c-1}\exp -x^c$ | $c = 4.362$, $y = \dfrac{x - 23.90}{4.222}$ | 0.19 | $3.9\times10^{-9}$ |
| $\gamma$ | $f(x,c) = \dfrac{c}{2\Gamma(1/c)}\exp -\lvert x\rvert^c$ | $c = 1.277$, $y = \dfrac{x - 1.94}{0.4042}$ | 0.99 | 0.16 |

Table S3: The fit for the properties of $Al_2O_3$ at 900K with the result of the Cramer von Mises (CVM) goodness of fit test and Vuong Test.

| Property | Form | | CVM | Vuong Test |
|---|---|---|---|---|
| $B_T$ | $f(x,c) = \frac{c}{2\Gamma(1/c)} \exp -\lvert x\rvert^c$ | $c = 1.856$ <br> $y = \frac{x - 185.3}{30.84}$ | 0.81 | 0.18 |
| $C_V$ | $f(y,a,c) = \frac{\lvert c\rvert x^{ca-1} \exp -x^c}{\Gamma(a)}$ | $a = 0.6456$ <br> $c = 5.537$ <br> $y = \frac{x - 115.8}{2.512}$ | 0.99 | 0.10 |
| $G$ | $f(y) = \phi(y)$ | $y = \frac{x + 31.57}{5.704}$ | 0.92 | 0.61 |
| $S$ | $f(y,a,c) = \frac{c}{\sqrt{y^2+1}} \phi(a + c\sinh^{-1}(y))$ | $a = -3.4619$ <br> $c = 3.967$ <br> $y = \frac{x - 151.5}{19.62}$ | 0.75 | 0.019 |
| $\Theta_D$ | $f(x,c) = \frac{c}{2\Gamma(1/c)} \exp -\lvert x\rvert^c$ | $c = 0.2561$ <br> $y = \frac{x - 923.3}{25.80}$ | 0.82 | $4.3\times10^{-3}$ |
| $\alpha_V$ | $f(y,a,c) = \frac{c}{\sqrt{y^2+1}} \phi(a + c\sinh^{-1}(y))$ | $a = -0.6466$ <br> $c = 1.4955$ <br> $y = \frac{x - 37.04}{14.15}$ | 0.99 | $4.2\times10^{-7}$ |
| $V$ | $f(y,c) = \frac{1}{cy\sqrt{2\pi}} \exp\left(-\frac{\log^2(x)}{2c^2}\right)$ | $c = 0.01314$ <br> $y = \frac{x + 55.29}{83.69}$ | 0.14 | $1.5\times10^{-6}$ |
| $\gamma$ | $f(x,c) = \frac{c}{2\Gamma(1/c)} \exp -\lvert x\rvert^c$ | $c = 1.277$ <br> $y = \frac{x - 1.94}{0.4042}$ | 0.99 | $1.9\times10^{-3}$ |

Table S4: The fit for the properties of NiO at 900K with the result of the Cramer von Mises (CVM) goodness of fit test and Vuong Test.

| Property | Form | | CVM | Vuong Test |
|---|---|---|---|---|
| $B_T$ | $f(y,a,c) = \frac{c}{\sqrt{y^2+1}}\phi(a + c\sinh^{-1}(y))$ | $a = 1.074$<br>$c = 2.876$<br>$y = \frac{x - 159.3}{86.57}$ | 0.71 | $8.0\times10^{-3}$ |
| $C_V$ | $f(y,c) = cx^{c-1}\exp -x^c$ | $c = 5.667$<br>$y = \frac{x - 48.178}{0.8557}$ | 0.97 | 0.63 |
| $G$ | $f(y,a,c) = \frac{c}{\sqrt{y^2+1}}\phi(a + c\sinh^{-1}(y))$ | $a = 2.799$<br>$c = 3.694$<br>$y = \frac{x - 28.77}{12.80}$ | 0.68 | 0.36 |
| $S$ | $f(y,a,c) = \frac{c}{\sqrt{y^2+1}}\phi(a + c\sinh^{-1}(y))$ | $a = -1.580$<br>$c = 1.614$<br>$y = \frac{x - 89.29}{6.747}$ | 0.52 | $1.0\times10^{-3}$ |
| $\Theta_D$ | $f(y,c) = c\phi(y)\Phi(-y)^{c-1}$ | $c = 0.6534$<br>$y = \frac{x - 531.8}{42.54}$ | 0.89 | 0.22 |
| $\alpha_V$ | $f(y,a,c) = \frac{c}{\sqrt{y^2+1}}\phi(a + c\sinh^{-1}(y))$ | $a = -0.8474$<br>$c = 0.9993$<br>$y = \frac{x - 29.06}{27.87}$ | 0.31 | $5.0\times10^{-22}$ |
| $V$ | $f(y,a,c) = \frac{c}{\sqrt{y^2+1}}\phi(a + c\sinh^{-1}(y))$ | $a = 1.179$<br>$c = 1.944$<br>$y = \frac{x - 11.98}{1.0966}$ | 0.0033 | 0.062 |
| $\gamma$ | $f(x,c) = \frac{c}{2\Gamma(1/c)}\exp -\|x\|^c$ | $c = 1.811$<br>$y = \frac{x - 1.910}{1.388}$ | 0.86 | 0.16 |

Table S5: The fit for the properties of Al at 300K with the result of the Cramer von Mises (CVM) goodness of fit test and Vuong Test.

| Property | Form | | CVM | Vuong Test |
|---|---|---|---|---|
| $B_T$ | $f(y,c) = 2\phi(y)\Phi(cy)$ | $c = -2.313$ <br> $y = \dfrac{x - 96.26}{25.43}$ | 0.46 | 0.0011 |
| $C_V$ | $f(y,c) = 2\phi(y)\Phi(cy)$ | $c = 2.526$ <br> $y = \dfrac{x - 21.96}{0.6211}$ | 0.61 | 0.025 |
| $G$ | $f(y,a,c) = \dfrac{c}{\sqrt{y^2+1}}\phi(a + c\sinh^{-1}(y))$ | $a = 2.818$ <br> $c = 2.172$ <br> $y = \dfrac{x - 2.187}{0.8558}$ | 0.47 | 0.15 |
| $S$ | $f(y,a,c) = \dfrac{c}{\sqrt{y^2+1}}\phi(a + c\sinh^{-1}(y))$ | $a = -2.853$ <br> $c = 1.897$ <br> $y = \dfrac{x - 21.49}{1.874}$ | 0.53 | 0.048 |
| $\Theta_D$ | $f(y,c) = 2\phi(y)\Phi(cy)$ | $c = -3.184$ <br> $y = \dfrac{x - 488.8}{62.28}$ | 0.65 | $5.7\times10^{-4}$ |
| $\alpha_V$ | $f(y,a,c) = \dfrac{c}{\sqrt{y^2+1}}\phi(a + c\sinh^{-1}(y))$ | $a = -2.148$ <br> $c = 1.251$ <br> $y = \dfrac{x - 29.31}{8.984}$ | 0.11 | $1.4\times10^{-4}$ |
| $V$ | $f(y,a,c) = \dfrac{c}{\sqrt{y^2+1}}\phi(a + c\sinh^{-1}(y))$ | $a = -2.497$ <br> $c = 3.532$ <br> $y = \dfrac{x - 8.782}{1.803}$ | 0.31 | 0.15 |
| $\gamma$ | $f(y,c) = 2\phi(y)\Phi(cy)$ | $c = 3.0160$ <br> $y = \dfrac{x - 1.472}{0.6813}$ | 0.11 | $1.4\times10^{-7}$ |

Table S6: The fit for the properties of Aluminium at 900K with the result of the Cramer von Mises (CVM) goodness of fit test and Vuong Test.

| Property | Form | | CVM | Vuong Test |
|---|---|---|---|---|
| $B_T$ | $f(y,c) = 2\phi(y)\Phi(cy)$ | $c = -3.602$ <br> $y = \dfrac{x - 92.63}{32.83}$ | 0.19 | $7.5\times10^{-5}$ |
| $C_V$ | $f(y,c) = 2\phi(y)\Phi(cy)$ | $c = 2.288$ <br> $y = \dfrac{x - 24.59}{0.07725}$ | 0.53 | 0.16 |
| $G$ | $f(y,a,c) = \dfrac{c}{\sqrt{y^2+1}}\phi(a + c\sinh^{-1}(y))$ | $a = 2.785$ <br> $c = 1.793$ <br> $y = \dfrac{x + 20.06}{1.868}$ | 0.55 | .33 |
| $S$ | $f(y,a,c) = \dfrac{c}{\sqrt{y^2+1}}\phi(a + c\sinh^{-1}(y))$ | $a = -2.550$ <br> $c = 1.424$ <br> $y = \dfrac{x - 48.62}{1.673}$ | 0.44 | $1.3\times10^{-3}$ |
| $\Theta_D$ | $f(y,c) = 2\phi(y)\Phi(cy)$ | $c = -3.184$ <br> $y = \dfrac{x - 488.8}{62.28}$ | 0.65 | $5.7\times10^{-4}$ |
| $\alpha_V$ | $f(y,a,c) = \dfrac{c}{\sqrt{y^2+1}}\phi(a + c\sinh^{-1}(y))$ | $a = -1.681$ <br> $c = 0.9107$ <br> $y = \dfrac{x - 138.05}{8.268}$ | 0.63 | $1.6\times10^{-10}$ |
| $V$ | $f(y,a,c) = \dfrac{c}{\sqrt{y^2+1}}\phi(a + c\sinh^{-1}(y))$ | $a = -2.4603$ <br> $c = 2.4417$ <br> $y = \dfrac{x - 9.033}{1.287}$ | 0.059 | 0.19 |
| $\gamma$ | $f(y,c) = 2\phi(y)\Phi(cy)$ | $c = 3.0160$ <br> $y = \dfrac{x - 1.472}{0.6813}$ | 0.11 | 0.014 |

(9) Seltz, H.; DeWitt, B. J.; McDonald, H. J. The Heat Capacity of Nickel Oxide from 68-298K. and the Thermodynamic Properties of the Oxide. *Journal of the American Chemical Society* **1940**, *62*, 88–89.

(10) Jifang, W.; Fisher, E. S.; Manghnzmi, M. H. Elastic Constants of Nickel Oxide. *Chinese Physics Letters* **1991**, *8*, 153–156.

(11) Madelung, O.; Rössler, U.; Schulz, M. Non-Tetrahedrally Bonded Binary Compounds II.

(12) Anderson, T. W.; Darling, D. A. Asymptotic theory of certain "goodness of fit" criteria based on stochastic processes. *Ann. Math. Stat.* **1952**, *23*, 193–212.

(13) Parks, H. L.; McGaughey, A. J. H.; Viswanathan, V. Uncertainty Quantification in First-Principles Predictions of Harmonic Vibrational Frequencies of Molecules and Molecular Complexes. *J. Phys. Chem. C* **2019**, *123*, 4072–4084.
